# Supplementary material for: Two and three electrons on a sphere: A generalized Thomson problem
Source: arXiv:1806.08315 source file (2018-06-21)
Supplement: Supplementary file 1 [file SI_resubmit.pdf]

# Two and three electrons on a sphere: A generalized Thomson problem – Supplemental Material

Liu Yang and Zhenwei Yao*

*School of Physics and Astronomy, and Institute of Natural Sciences, Shanghai Jiao Tong University, Shanghai 200240, China*

In this Supplemental Material we provide the details of some results in the main text.

## I. THE CASE OF A SINGLE ELECTRON

For a single electron on the sphere, $\hat{K} = -\frac{\hbar^2}{2m_e}\nabla^2$, where $\nabla^2 = \frac{1}{R^2 \sin\theta}(\frac{\partial}{\partial\theta}\sin\theta\frac{\partial}{\partial\theta}) + \frac{1}{R^2\sin^2\theta}\frac{\partial^2}{\partial\phi^2}$ in the spherical coordinates. $\theta \in [0, \pi]$, and $\phi \in [0, 2\pi)$. The solution to the energy eigenvalue equation Eq.(1) in the main text is [1]:

$$\Psi_l^m(\theta, \phi) = \frac{1}{R}\sqrt{\frac{(2l+1)(l-m)!}{2\pi(l+m)!}}P_l^m(\cos\theta) \times \{\cos m\phi, \sin m\phi\}, \tag{I.1}$$

where the angular momentum quantum number $l$ is a nonnegative integer, and $m = 0, 1, 2...l$. The energy eigenvalue $E_l = \hbar^2 l(l+1)/2MR^2$. Note that $E_l$ is independent on $m$.

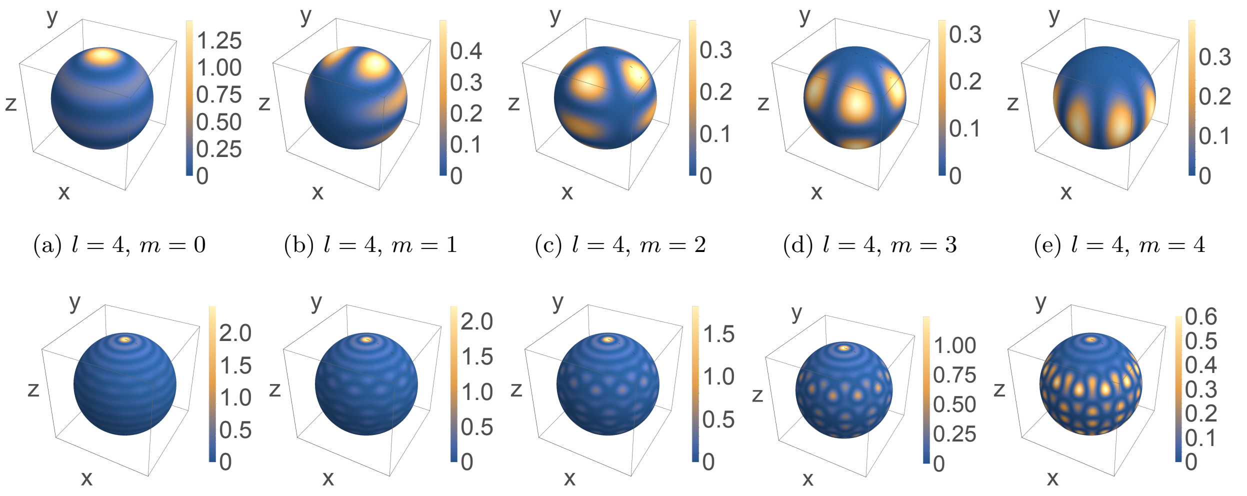


(a) $l = 4$, $m = 0$ (b) $l = 4$, $m = 1$ (c) $l = 4$, $m = 2$ (d) $l = 4$, $m = 3$ (e) $l = 4$, $m = 4$

(f) $c = 0.1$ (g) $c = 0.3$ (h) $c = 0.5$ (i) $c = 0.7$ (j) $c = 0.9$

FIG. 1: Self-interference patterns of a single electron confined on the surface of a sphere. (a)-(e): the probability density distribution $\rho_{lm}(\theta, \phi) = |\Psi_l^m(\theta, \phi)|^2$. (f)-(j): the probability density distribution of the following superposition state at varying $c$: $\Psi(\theta, \phi) = \sqrt{1-c^2}\Psi_l^0(\theta, \phi) + c\Psi_l^m(\theta, \phi)$. $l = 15$, and $m = 12$.

*Electronic address: zyao@sjtu.edu.cn

Figure 1 shows the probability density distribution $\rho_{lm}(\theta,\phi) = |\Psi_l^m(\theta,\phi)|^2$. In Figs. 1(a)-1(e), $\ell$ is fixed, and $m$ varies from 0 to $\ell$. The $m = 0$ state exhibits the axisymmetric layered structure. The electron has the largest probability to appear at the poles of the sphere [see the brightest regions in Fig. 1]. With the increase of $m$, the rotational symmetry of the self-interference pattern evolves from $C_\infty$ ($m = 0$), $C_2(m = 1)$, $C_4(m = 2)$, $C_6(m = 3)$ to $C_8$ symmetry ($m = 4$). At $m = l$, the electron tends to appear at $2m$ discrete spots around the equatorial region of the sphere.

We notice that, for any state $\Psi_l^m(\theta,\phi)$, the probability density distribution is peaked around $l - m + 1$ circles of latitude, and $2m$ circles of longitude. This property suggests that one may fabricate self-interference patterns of a single electron by a linear superposition of energetically degenerate wave functions $\Psi_l^m(\theta,\phi)$. In Figs. 1(f)-1(j), we show the probability density distribution of the following superposition state at varying $c$: $\Psi(\theta,\phi) = \sqrt{1-c^2}\Psi_l^0(\theta,\phi)+c\Psi_l^m(\theta,\phi)$. We see the evolution of the belt structure near the equator [see Fig. 1(f)] to a triangular lattice [see Fig. 1(j)] with the increase of $c$.

## II. SYMMETRIZED BASES OF $\mathscr{H}(1,0)$ FOR THE TWO-ELECTRON SYSTEM

The symmetrized bases $\varepsilon^{X_p}(l = 1, m = 0)$ of the subspace $\mathscr{H}(l = 1, m = 0)$ for the two-electron system is denoted as $\Psi_i^{X_p}(\vec{r}_1,\vec{r}_2)$. The superscript $X_p$ indicates that the wave function is exchange-symmetric ($X = S$) or exchange-antisymmetric ($X = A$), and has even ($p = e$) or odd ($p = o$) parity. The subscript $i$ completely determines the quantum number set $\{l_1, l_2, l, m\}$ of the state in $\varepsilon^{X_p}(l, m)$. . The expressions for the three kinds of symmetrized bases are:

$$\begin{aligned}\Psi_i^{S_o}(\vec{r}_1,\vec{r}_2) &= \frac{1}{\sqrt{2}}\langle\vec{r}_1,\vec{r}_2|(|i,i+1,1,0\rangle + |i+1,i,1,0\rangle)\\ &= \frac{1}{\sqrt{2}}\sum_{m=-i}^{m=i}(Y_i^m(\theta_1,\phi_1)Y_{i+1}^{-m}(\theta_2,\phi_2) + Y_i^m(\theta_2,\phi_2)Y_{i+1}^{-m}(\theta_1,\phi_1))C_{m,-m,0}^{i,i+1,1},\end{aligned} \tag{II.1}$$

$$\Psi_i^{A_e}(\vec{r}_1,\vec{r}_2) = \langle\vec{r}_1,\vec{r}_2|i,i,1,0\rangle = \sum_{m=-i}^{m=i} Y_i^m(\theta_1,\phi_1)Y_i^{-m}(\theta_2,\phi_2)C_{m,-m,0}^{i,i,1}, \tag{II.2}$$

$$\begin{aligned}\Psi_i^{A_o}(\vec{r}_1,\vec{r}_2) &= \frac{1}{\sqrt{2}}\langle\vec{r}_1,\vec{r}_2|(|i,i+1,1,0\rangle - |i+1,i,1,0\rangle)\\ &= \frac{1}{\sqrt{2}}\sum_{m=-i}^{m=i}(Y_i^m(\theta_1,\phi_1)Y_{i+1}^{-m}(\theta_2,\phi_2) - Y_i^m(\theta_2,\phi_2)Y_{i+1}^{-m}(\theta_1,\phi_1))C_{m,-m,0}^{i,i+1,1}.\end{aligned} \tag{II.3}$$

$C^{l_1 l_2 l}_{m_1 m_2 m}$ is the Clebsch-Gordan coefficient:

$$C^{l_1 l_2 l}_{m_1 m_2 m} = \langle l_1, m_1; l_2, m_2 | l_1, l_2, l, m\rangle \tag{II.4}$$

$$= (-1)^{l_1+l_2+m}\sqrt{2l+1}\begin{pmatrix} l_1 & l_2 & l \\ m_1 & m_2 & -m \end{pmatrix}, \tag{II.5}$$

where $\begin{pmatrix} l_1 & l_2 & l \\ m_1 & m_2 & -m \end{pmatrix}$ is the Wigner 3-j symbols [2].

Note that no base of the subspace $\mathscr{H}(1,0)$ is both exchange-symmetric and with even parity. In fact, any wave function in $\mathscr{H}(1,0)$ with even parity must be exchange-antisymmetric. To prove this claim, we first show that for a even base wave function in $\mathscr{H}(1,0)$, $l_1$ must be equal to $l_2$ such that both conditions of $l_1+l_2$ are even and $|l_1-l_2| \leq 1 \leq l_1+l_2$ are satisfied. By applying the relation of $C^{l_1,l_2,l}_{m_1,m_2,m} = -C^{l_2,l_1,l}_{m_2,m_1,m}$ to the case of $l=1,\ m=0$, we have $\langle \vec{r}_1, \vec{r}_2 | l_1, l_1, 1, 0\rangle = -\langle \vec{r}_2, \vec{r}_1 | l_1, l_1, 1, 0\rangle$. That is, for the wave function with even parity in $\mathscr{H}(1,0)$, exchanging the electrons' positions will change the sign of the wave function, indicating the exchange-antisymmetric nature of the wave function.

## III. ADDITION OF ANGULAR MOMENTUMS IN THE THREE-ELECTRON SYSTEM

For the three-electron system, $\hat{L}^2_{12}$, $\hat{L}^2_1$, $\hat{L}^2_2$, $\hat{L}^2_3$, $\hat{L}^2$, $\hat{L}_z$ commute with each other. To construct their common eigen state $|l_{12}, l_1, l_2, l_3, l, m\rangle$, we first consider addition of angular momentums of two electrons. The common eigen state of the mutually commuting operators $\hat{L}^2_{12}$, $\hat{L}^2_1$, $\hat{L}^2_2$, and $\hat{L}_{12z}$ of the two-electron system is:

$$|l_1, l_2, l_{12}, m_{12}\rangle = \sum_{m_1=-l_1}^{l_1}\sum_{m_2=-l_2}^{l_2} |l_1, m_1; l_2, m_2\rangle\langle l_1, m_1; l_2, m_2 | l_1, l_2, l_{12}, m_{12}\rangle, \tag{III.1}$$

where $|l_1, m_1; l_2, m_2\rangle = |l_1, m_1\rangle \otimes |l_2, m_2\rangle$.

By further adding the angular momentum of the third electron, we have

$$|l_{12}, l_1, l_2, l_3, l, m\rangle = \sum_{m_{12}=-l_{12}}^{l_{12}}\sum_{m_3=-l_3}^{l_3} |l_1, l_2, l_{12}, m_{12}; l_3, m_3\rangle\langle l_1, l_2, l_{12}, m_{12}; l_3, m_3 | l_{12}, l_1, l_2, l_3, l, m\rangle \tag{III.2}$$

The coefficient $\langle l_1, l_2, l_{12}, m_{12}; l_3, m_3 | l_{12}, l_1, l_2, l_3, l, m\rangle$ is recognized as $\langle l_{12}, m_{12}; l_3, m_3 | l_{12}, l_3, l, m\rangle$

due to the normalization condition of $\langle l_1, l_2 | l_1, l_2\rangle = 1$. We thus have

$$\begin{aligned}\Psi_{\mathbf{n}}(\vec{r}_1, \vec{r}_2, \vec{r}_3) =& \langle \vec{r}_1, \vec{r}_2, \vec{r}_3 | l_{12}, l_1, l_2, l_3, l, m\rangle \\ =& \frac{1}{R^3} \sum_{m_1=-l_1}^{l_1} \sum_{m_2=-l_2}^{l_2} \sum_{m_3=-l_3}^{l_3} C^{l_{12}, l_1, l_2, l_3, l}_{m_1, m_2, m_3, m} Y^{m_1}_{l_1}(\vec{n}_1) Y^{m_2}_{l_2}(\vec{n}_2) Y^{m_3}_{l_3}(\vec{n}_3),\end{aligned} \tag{III.3}$$

where $|\mathbf{n}\rangle = |l_{12}, l_1, l_2, l_3, l, m\rangle$, and

$$C^{l_{12}, l_1, l_2, l_3, l}_{m_1, m_2, m_3, m} = \langle l_1, m_1; l_2, m_2 | l_1, l_2, l_{12}, m_1 + m_2\rangle \langle l_{12}, m_1 + m_2; l_3, m_3 | l_{12}, l_3, l, m\rangle$$

In our work, we focus on solving the ground state wave functions in the subspace $\mathscr{H}(l = 0, m = 0)$ spanned by the basis set $\varepsilon(0, 0) = \{|l_{12} = l_3, l_1, l_2, l_3, l = 0, m = 0\rangle\}$, where $l_1, l_2, l_3 = 0, 1, 2, ...$, and $|l_1 - l_2| \le l_3 \le l_1 + l_2$. The basis set $\varepsilon(0, 0)$ is determined by the three quantum numbers $l_1, l_2$ and $l_3$, which are denoted as $\mathbf{L} = (l_1, l_2, l_3)$. From Eq.(III.3), we obtain the associated eigen state wave function:

$$\Psi_{\mathbf{L}}(\vec{r}_1, \vec{r}_2, \vec{r}_3) = \frac{1}{R^3} \sum_{m_1=-l_1}^{l_1} \sum_{m_2=-l_2}^{l_2} \begin{pmatrix} l_1 & l_2 & l_3 \\ m_1 & m_2 & -m_1 - m_2 \end{pmatrix} Y^{m_1}_{l_1}(\vec{r}_1) Y^{m_2}_{l_2}(\vec{r}_2) Y^{-m_1-m_2}_{l_3}(\vec{r}_3) \tag{III.4}$$

## IV. SMALL OSCILLATION THEORY FOR THE THREE-ELECTRON SYSTEM

In the large-$R$ regime, energetics and probability analysis presented in the main text have shown the localization of the three electrons near the vertices of a regular triangle circumscribed by the equator of the sphere. We employ the small oscillation theory to analyze the vibration of the electrons around the equilibrium positions at $(\bar{\theta}_1 = \pi/2, \bar{\phi}_1 = 0)$, $(\bar{\theta}_2 = \pi/2, \bar{\phi}_2 = 2\pi/3)$, and $(\bar{\theta}_3 = \pi/2, \bar{\phi}_3 = 4\pi/3)$ [3]. The classical Hamiltonian of our system is

$$H = \frac{1}{2} R^2 \sum_{i=1}^{3} (\delta\dot{\theta}_i^2 + \delta\dot{\phi}_i^2) + \sum_{i,j=1}^{3} (\delta\theta_i \delta\theta_j Q^1_{ij} + \delta\phi_i \delta\phi_j Q^2_{ij}) + \frac{\sqrt{3}}{R}, \tag{IV.1}$$

where

$$Q^1 = \frac{1}{6\sqrt{3}R} \begin{pmatrix} 1 & 1 & 1 \\ 1 & 1 & 1 \\ 1 & 1 & 1 \end{pmatrix}, \quad Q^2 = \frac{5}{24\sqrt{3}R} \begin{pmatrix} 2 & -1 & -1 \\ -1 & 2 & -1 \\ -1 & -1 & 2 \end{pmatrix}.$$

Through the following orthogonal transformation

$$\eta_1 = \frac{1}{\sqrt{3}}(\delta\theta_1 + \delta\theta_2 + \delta\theta_3), \qquad \eta_4 = \frac{1}{\sqrt{3}}(\delta\phi_1 + \delta\phi_2 + \delta\phi_3),$$
$$\eta_2 = \frac{1}{\sqrt{2}}(\delta\phi_2 - \delta\phi_1), \qquad \eta_5 = \frac{1}{\sqrt{2}}(\delta\theta_2 - \delta\theta_1),$$
$$\eta_3 = \frac{1}{\sqrt{2}}(\delta\phi_3 - \delta\phi_1), \qquad \eta_6 = \frac{1}{\sqrt{2}}(\delta\theta_3 - \delta\theta_1). \tag{IV.2}$$

the Hamiltonian is simplified to

$$H = \frac{1}{2}R^2\sum_{r=1}^{6}\dot{\eta}_r^2 + \frac{1}{2}\sum_{r=1}^{3}\omega_r^2 R^2\eta_r^2 + \frac{\sqrt{3}}{R}. \tag{IV.3}$$

The vibration frequencies are

$$\omega_1 = 3^{-\frac{1}{4}}R^{-\frac{3}{2}},$$
$$\omega_2 = \frac{\sqrt{5}}{2}3^{-\frac{1}{4}}R^{-\frac{3}{2}},$$
$$\omega_3 = \frac{\sqrt{5}}{2}3^{-\frac{1}{4}}R^{-\frac{3}{2}}. \tag{IV.4}$$

In the orthogonal transformation defined in Eq.(IV.2), $\eta_1$ and $\eta_2$ describe relative in-plane vibration between any two electrons, $\eta_1$ describes out-of-plane vibration, and the remaining collective coordinates describe the rotation of the whole system along x-, y-, and z-axis, respectively.

By promoting $R\dot{\eta}_r$ in Eq.(IV.3) to $-i\hbar\partial/(R\partial\eta_r)$, we obtain the quantized Hamiltonian:

$$\hat{H} = \sum_{r=1}^{6} -\frac{\hbar^2}{2R^2}\frac{\partial^2}{\partial\eta_r^2} + \frac{1}{2}\sum_{r=1}^{3}\omega_r^2 R^2\eta_r^2 + \frac{\sqrt{3}}{R}. \tag{IV.5}$$

The first three terms in the first sum term in Eq.(IV.5), in combination with the second sum term, constitute the Hamiltonian of three one-dimensional quantum harmonic oscillators. The terms associated with $\eta_4$, $\eta_5$ and $\eta_6$ in Eq.(IV.5) describe free particles confined on the sphere of radius $R$.

The eigen energy of a one-dimensional oscillator characterized by $\eta_r$ is $(n_r+1/2)\hbar\omega_r$ $(r = 1, 2, 3)$, and the rotational energy associated with $\eta_i$ $(i = 4, 5, 6)$ has the form of $L_i(L_i + 1)\hbar^2/R^2$ ($L_i$ is an integer). In the large-$R$ regime, since the former and latter energy scales with $R$ in the form of $R^{-3/2}$ and $R^{-2}$ respectively, one can neglect the rotational energy when analyzing the vibrational modes.

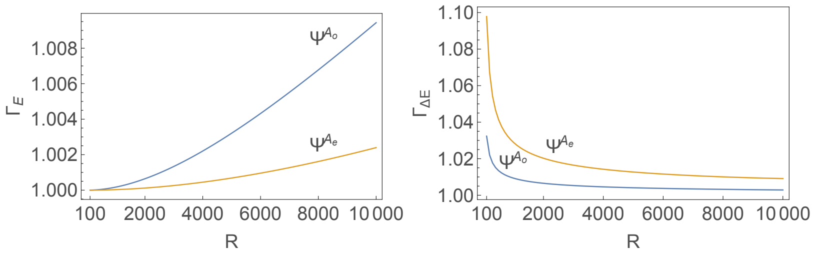


(a) (b)

FIG. 2: Illustration of the accuracuy of the perturbation analysis and the small oscillation theory in the small- and large-$R$ regimes. $\Gamma_E$ is the ratio of the ground state energy derived from the perturbation theory (up to the first-order correction) and that from the CI method. $\Gamma_{\Delta E}$ is the ratio of the ground state energy (substracted by $\sqrt{3}/R$) obtained from the small oscillation theory and that from the CI method.

| R | $E^{\rm CI}$ | $E^{\rm exact}$ |
|---|---|---|
| 0.01 | 99.773785103 | 99.773761078 |
| 0.1 | 9.783893797 | 9.783873673 |
| 0.5 | 1.820610326 | 1.820600768 |
| 1 | 0.852785205 | 0.852781065 |
| 5 | 0.139470864 | 0.139470826 |
| 10 | 0.064525124 | 0.064525123 |
| 100 | 0.005487412 | 0.005487412 |
| 1000 | 0.000515686 | 0.000515686 |

TABLE I: Comparison of our CI results $E^{\rm CI}$ for the ground state energy of the $\Psi^{S_e}$ state with the exact results $E^{\rm exact}$ in Ref. [4]. The same digits in the two columns are colored in red.

## V. ACCURACY OF PERTURBATION ANALYSIS AND SMALL OSCILLATION THEORY

To check the accuracy of perturbation analysis in the small-$R$ regime, we compare the ground state energy derived from the perturbation theory (up to the first-order correction) with that from the CI method. Their ratio is denoted as $\Gamma_E$. From Fig.2(a), we see that for both cases of $\Psi^{A_o}$ and $\Psi^{A_e}$, the maximum $\Gamma_E$ is less than 1% in the interested regime of $R \leq 1$.

Similarly, the accuracy of the small oscillation theory in the large-$R$ regime is measured by the ratio $\Gamma_{\Delta E}$ of the ground state energy (subtracted by $\sqrt{3}/R$) obtained from the small oscillation theory and that from the CI method. Fig.2(b) shows that the value of $\Gamma_{\Delta E}$ is very close to unity, especially in the large-$R$ end.

## VI. PRECISION OF OUR NUMERICAL RESULTS BASED ON THE CI METHOD

In Table I, we compare our numerical results for the ground state energy of the $\Psi^{S_e}$ state with the exact values in Ref. [4] at various $R$. Furthermore, we compare our numerical result for the ground state energy of the $\Psi^{S_e}$ state with the available analytical value in Ref. [5] for the case of $R = \sqrt{3}/2$. The analytical value is 1, and our result is 1.0000051.


[1] G. B. Arfken, *Mathematical methods for physicists* (Academic Press, 1985), 3rd ed.

[2] L.D.Landau and E.M.Lifshitz, *Quantum Mechanics* (Butterworth-Heinemann, 1981), 3rd ed.

[3] H. Goldstein, *Classical mechanics* (Pearson Education India, 2011).

[4] P.-F. Loos and P. M. W. Gill, Phys. Rev. A **79**, 062517 (2009).

[5] P.-F. Loos and P. M. Gill, Phys. Rev. Lett. **103**, 123008 (2009).
